# Supplementary material for: FedNest: Federated Bilevel, Minimax, and Compositional Optimization
Source: arXiv:2205.02215 source file (2022-09-13)
Supplement: Supplementary file 1 [file supp_algotable.tex]

\begin{table*}[t]
\centering
\scalebox{0.8}{
\begin{tabular}{lccccccc}
\toprule 
 & \multicolumn{2}{c}{definition} & & \multicolumn{4}{c}{properties} \\ \cmidrule{2-3}\cmidrule{5-8} 
                            & inner & outer  & & global & global & local & \#comm. \\
                       & optimization  & optimization & & gradient & IHGP& steps & rounds \\
                       \midrule
\pmb{\fedblo}  &   Alg.~\ref{alg:fedout}              &  Alg.~\ref{algo:svrg}                              &    & yes             &   yes              & no          & 3                      \\
\pmb{\fedblo} with local \fedout and  SVRG & Alg.~\ref{alg:GIANT_local_steps-local} & Alg.~\ref{alg:GIANT-linesearch} & & yes            &    yes              & yes         & 3                      \\
%GIANT with local steps & \multirow{2}{*}{Alg.~\ref{alg:GIANT_local_steps-local}} & \multirow{2}{*}{Alg.~\ref{alg:GIANT-linesearch}} & & \multirow{2}{*}{yes}            &    \multirow{2}{*}{yes}              & \multirow{2}{*}{yes}         & \multirow{2}{*}{3}                      \\
%and global line search &              &                 &          &                       \\
\pmb{\fedblo} with local \fedout and  SGD & Alg.~\ref{alg:GIANT_local_steps_local_linesearch-local} & Alg.~\ref{alg:local_linesearch-update} & & yes             &   no               & yes         & 2                      \\
%GIANT with local steps  & \multirow{2}{*}{Alg.~\ref{alg:GIANT_local_steps_local_linesearch-local}} & \multirow{2}{*}{Alg.~\ref{alg:local_linesearch-update}} & & \multirow{2}{*}{yes}             &   \multirow{2}{*}{no}               & \multirow{2}{*}{yes}         & \multirow{2}{*}{2}                      \\
%and local line search &              &                 &          &                       \\
\pmb{\fedblo} with local \fedout and local outer SGDxw & Alg.~\ref{alg:LocalNewton_global_linesearch-local} & Alg.~\ref{alg:LocalNewton-linesearch}     &  & no & yes & yes & 2 \\
%LocalNewton with     & \multirow{2}{*}{Alg.~\ref{alg:LocalNewton_global_linesearch-local}} & \multirow{2}{*}{Alg.~\ref{alg:LocalNewton-linesearch}}     &  & \multirow{2}{*}{no}              &   \multirow{2}{*}{yes}              & \multirow{2}{*}{yes}         & \multirow{2}{*}{2 (3)}                  \\
%global line search &              &                 &          &                       \\
  &  Alg.~\ref{alg:LocalNewton-local}                 &  Alg.~\ref{alg:local_linesearch-update}     & & no              &   no               & yes         & 1  \\ \bottomrule
\end{tabular}
}
\caption{Definition of studied algorithms by used local optimization algorithms and server updates and resulting properties of these algorithms.}
\label{tabl:supp:methods}
%\vspace{-0.5mm}
\end{table*}
