# Supplementary material for: FedNest: Federated Bilevel, Minimax, and Compositional Optimization
Source: arXiv:2205.02215 source file (2022-09-13)
Supplement: Supplementary file 3 [file supp_extra.tex]

\section{Federated Bi-Level Learning and \fedblo}\label{sec:fedavg}
In federated bilevel learning, we solve an optimization problem of the form: 
\begin{align}\label{fedblo:prob}
\begin{array}{ll}
\underset{\m{x} \in \mb{R}^{{d}_1}}{\text{minimize}} &
\begin{array}{c}
\hspace{.1cm} \frac{1}{n_1} \sum_{i=1}^{n_1} f_i\left(\m{x},\m{y}^*(\m{x})\right)
\end{array}\\
\text{subj.~to} & \begin{array}[t]{l}
\hspace{.2cm}  \m{y}^*(\m{\m{x}})=\underset{ \m{y}\in \mb{R}^{{d}_2}}{\textnormal{argmin}}~~\frac{1}{n_2}\sum_{i=1}^{n_2} g_i\left(\m{x},\m{y}\right).
\end{array}
\end{array}
\end{align}
Here, the components $\{f_i\}_{i=1}^{n_1}$ and $\{g_i\}_{i=1}^{n_2}$ are distributed among $n_1$ and $n_2$ clients, respectively. For simplicity, we set $n:=n_1=n_2$. Throughout, we make the following assumptions.

\begin{assumption}\label{assu:f} 
%\noindent   {\bf Assumptions A}
For all $i \in [n]$:
\begin{enumerate}[label={\textbf{(A\arabic*})}]
%[label={\textbf{(a\arabic*})}]
\item %[\textbf{a)}]
% \noindent\textbf{Assumption 1 (Lipschitz continuity).}
%%Function $f(x,y)$ is differentiable, $g(x,y)$ is twice differentiable.  
%For any fixed $x$, $\nabla_x f(x,\cdot)$, $\nabla_y f(x,\cdot)$, $\nabla_y g(x,\cdot)$, $\nabla^2_{xy}g(x,\cdot)$, $\nabla^2_{yy}g(x,\cdot)$ are $L_{f_x}, L_{f_y}, L_g, L_{g_{xy}}, L_{g_{yy}}$-Lipschitz continuous. For any fixed $y$, $\nabla_x f(\cdot, y)$, $\nabla_y f(\cdot, y)$, $\nabla^2_{xy}g(\cdot, y)$, $\nabla^2_{yy}g(\cdot, y)$ are $\bar L_{f_x}, \bar L_{f_y}, \bar L_{g_{xy}}, \bar L_{g_{yy}}$-Lipschitz continuous.}  
$f_i, \nabla f_i, \nabla g_i, \nabla^2 g_i$ are respectively $\ell_{f,0}$, $\ell_{f,1}, \ell_{g,1}, \ell_{g,2}$-Lipschitz continuous. 
% that is, for $\m{w}_1:=[\m{x}_1;\m{y}_1]$, $\m{z}_2:=[x_2;y_2]$, we have $\|f(x_1,y_1)-f(x_2,y_2)\|\leq \ell_{f,0}\|z_1-z_2\|, \|\nabla f(x_1,y_1)-\nabla f(x_2,y_2)\|\leq \ell_{f,1}\|z_1-z_2\|, \|\nabla g(x_1,y_1)-\nabla g(x_2,y_2)\|\leq \ell_{g,1}\|z_1-z_2\|, \|\nabla^2 g(x_1,y_1)-\nabla^2 g(x_2,y_2)\|\leq \ell_{g,2}\|z_1-z_2\|$.
% For any $\m{x} \in \mb{R}^{d_1}$, $\nabla_\m{x} f_t(\m{x},\m{y})$, $\nabla_\m{y} f_t(\m{x},\m{y})$, $\nabla_\m{y}  g_t(\m{x},\m{y})$, $\nabla_{\m{x}\m{y}} ^2g_t(\m{x},\m{y})$ and $\nabla_{\m{y}\m{y}} ^2g(\m{x},\m{y})$ are Lipschitz continuous with respect to $\m{y}$ with Lipschitz parameter  $L_{f_\m{x}}$, $L_{f_\m{y}}$, $L_{g_{\m{y}}}$, $L_{g_{\m{x}\m{y}}}$ and $L_{g_{\m{y}\m{y}}}$, respectively. 
% \item %[\textbf{b)}]
% For any given $\m{y} \in \mathbb{R}^{d_2}$,  $\nabla_\m{y}  f_t(\m{x},\m{y})$,  $\nabla_{\m{x}\m{y}} ^2g_t(\m{x},\m{y})$ and $\nabla_{\m{y}\m{y}} ^2g_t(\m{x},\m{y})$ are Lipschitz continuous with respect to $\m{x}$ with positive constants  $\wh{L}_{f_\m{y}}$, $\wh{L}_{g_{\m{x}\m{y}}}$ and $\wh{L}_{g_{\m{y}\m{y}}}$, respectively. 
% \item % [\textbf{c)}]
% 	For all $\m{x}\in \mc{X}$ and $\m{y} \in \mathbb{R}^n$, it holds that $\|\nabla_\m{y}  f_t(\m{x},\m{y})\|\leq C_{\m{y}}$ and 
% 	$\|\nabla_{\m{x}\m{y}} ^2 g_t(\m{x},\m{y})\|\leq C_{\m{x}\m{y}}$ for some constants $C_{\m{y}}$ and $C_{\m{x}\m{y}}$.
\item % [\textbf{d)}]
$g_i(\m{x},\m{y})$ is $\mu_{g}$-strongly convex in $\m{y}$ for any fixed $\m{x}\in \mc{X}$.
\end{enumerate}
\end{assumption}

% \begin{enumerate}[label={\textbf{B\arabic*}.}]
% \item  \label{assu:b1} %[\textbf{a)}]
% For any ${\m{x}} \in \mb{R}^{d_1}$, $\nabla_{\m{x}} f_i({\m{x}},{y})$, $\nabla_{y} f_i({\m{x}},{y})$, $\nabla_{y}  g_i({\m{x}},{y})$, $\nabla_{{\m{x}}{y}} ^2g_i({\m{x}},{y})$ and $\nabla_{{y}{y}} ^2g_i({\m{x}},{y})$ are Lipschitz continuous with respect to ${y}$ with Lipschitz parameter  $L_{f_{i,\m{x}}}$, $L_{f_{i,y}}$, $L_{g_{i,y}}$, $L_{g_{i,{\m{x}}{y}}}$ and $L_{g_{i,{y}{y}}}$, respectively. 

% \item \label{assu:b2} %[\textbf{b)}]
% For any given ${y} \in \mb{R}^{d_2}$, $\nabla_{\m{x}}  f_i({\m{x}},{y})$,  $\nabla_{y}  f_i({\m{x}},{y})$,  $\nabla_{{\m{x}}{y}} ^2g_i({\m{x}},{y})$ and $\nabla_{{y}{y}} ^2g_i({\m{x}},{y})$ are Lipschitz continuous with respect to ${\m{x}}$ with positive constants  $\wh{L}_{f_{i,\m{x}}}$, $\wh{L}_{f_{i,y}}$, $\wh{L}_{g_{i,{\m{x}}{y}}}$ and $\wh{L}_{g_{i,{y}{y}}}$, respectively. 
% \item  \label{assu:b3} % [\textbf{c)}]
% 	For all ${\m{x}}\in \mc{X}$ and ${y} \in \mb{R}^n$, it holds that $\|\nabla_{y}  f_i({\m{x}},{y})\|\leq C_{f_{i,y}}$ and 
% 	$\|\nabla^2_{{\m{x}}{y}}g_i({\m{x}},{y})\|\leq C_{g_{i,xy}}$ for some constants $C_{f_{i,y}}$ and $C_{g_{i,xy}}$.
% \item \label{assu:b4} % [\textbf{d)}]
% The inner function $g_i({\m{x}},{y})$ is $\mu_{g_i}$-strongly convex in ${y}$ for any ${\m{x}}\in \mc{X}$.
% \end{enumerate}
% \end{assumption}

Next, we discuss how to define an appropriate approximation for the  gradient  of  the objective function $f$ in the outer problem. To do so, we recall how the \emph{implicit differentiation} formula of the gradient $\nabla \m{y}^*(\m{x})$ is obtained for smooth inner optimization problems \citep{bengio2000gradient}. The proof is provided in Appendix. 

% We will provide a generalization to non-smooth optimization problems in \Cref{sub:implicit_nonsmooth}.
%
\begin{lemma}\label{thm:smooth_implicitdiff}
Under Assumptions~\ref{assu:f}, we have
\begin{align} \label{eq:grad_smooth}
    \nabla f_i(\m{x}, \m{y}^*(\m{x})) & = \nabla_{\m{x}}f_i\left(\m{x},\m{y}^*(\m{x})\right) +    \nabla \m{y}^*(\m{x}) \nabla_\m{y} f_i \left(\m{x},\m{y}^*(\m{x})\right),
    \end{align}
where
\begin{align}
   \nabla \m{y}^*(\m{x})=-\bigg(\sum_{j=1}^n \nabla^2_{xy}g_j\left(\m{x},\m{y}^*(\m{x})\right)\bigg) \bigg( \sum_{j=1}^n\nabla_{\m{y}}^2 {g_j}(\m{x},\m{y}^*(\m{x}))\bigg)^{-1}
\end{align}
\end{lemma}

To provide an iterative algorithm for solving problem \eqref{fedblo:prob}, we typically need to compute the gradient of $f$ at a given point $\m{x} \in  \mb{R}^{{d}_1}$ which requires knowing is not available unless the inner problem has a closed-form solution which is only possible for very specific choices
of function $g$. Therefore, we assume that for any $\m{x} \in  \mb{R}^{{d}_1}$, we have an approximation of $\m{y}^*(\m{x})$ which is used to estimate the gradient of $f$ at $\m{x}$. More specifically, for any $\m{x} \in  \mb{R}^{{d}_1}$, we define the gradient approximation of $f$ as
\begin{eqnarray}    \label{eq:approximate-gradient-nodewise}
\widetilde{\nabla} f_i\left(\m{x}_i,\tilde y_i\right) &:=& \nabla_{\m{x}}f_i\left(\m{x}_i,\tilde y_i\right)-
J_{i,w,\tau} (\m{x}_i,\tilde y_i) H^{-1}_{i,w,\tau} \left(\m{x}_i,\tilde y_i\right)
  \nabla_y f_i \left(\m{x}_i,\tilde y_i\right) 
  \nonumber \\
  &=& \nabla_{\m{x}}f_i\left(\m{x}_i,\tilde y_i\right)-
M_{i,w,\tau} (\m{x}_i,\tilde y_i) 
  \nabla_y f_i \left(\m{x}_i,\tilde y_i\right) 
\end{eqnarray}

% {
% \small
% \begin{algorithm}[htb]
% \caption{\pmb{\fedopt} (\m{x}, \m{y})}
% \label{alg:generalized_fedavg}
% \begin{algorithmic}[1]
% 	 %   \State Input: $y=\m{y}$
% %	    \For{$t = 0, \cdots, T-1$}
%     	    \State Sample a subset $\mathcal{S}$ of clients
%     	    \State $\m{y}^t_{i,0} = \m{y}_{t}$
%     	    \For{each client $i \in \mathcal{S}$ \textbf{in parallel}}
%         	    \For {$k = 0, \cdots, K-1$}
%             	    \State Compute an unbiased estimate $g_{i,k}^t$ of $\nabla g_i(\m{x}, \m{y}^t_{i,k})$
%             	    \State $\m{y}_{i,k+1}^t = \m{y}_{i, k}^t - \beta_l g_{i,k}^t$
%         	    \EndFor
%         	   % \State $\Delta_i^t = \m{y}^t_{i, K} - \m{y}_{t}$
%     	    \EndFor
%     	    \State $\m{y}_{t+1} = \frac{1}{|\mathcal{S}|}\sum_{i \in \mathcal{S}} \m{y}_{i}^t$
% 	%	\EndFor
% \end{algorithmic}
% \label{alg:fedopt}
% \end{algorithm}
% }

{
\small
\begin{algorithm}[htb]
\caption{$\m{y}^{T}~=~\pmb{\fedopt} (\m{x}, \m{y}^0, \beta)$}
\label{alg:generalized_fedavg}
\begin{algorithmic}[1]
	    %\State Input: 
	    \For{$t=0,\cdots,T-1$}
    	    \State Sample a subset $\mathcal{H}$ of clients
    	    \State $\m{y}_{i,0}^t = \m{y}^t$
    	    \For{each client $i \in \mathcal{H}$ \textbf{in parallel}}
        	    \For {$e = 0, \cdots, E-1$}
            	   % \State Compute an unbiased estimate $\m{g}_{i,e}$ of $\nabla g_i(\m{x}, \m{y}_{i,e})$
            	    \State $\m{y}_{i,e+1}^t=\m{y}_{i,e}^t-\beta \nabla g_i(\m{x}, \m{y}_{i,e}, \mc{S}_{i}^t)$
            	    \For {$e = 0, \cdots, E-1$}
            	    \State Compute an unbiased estimate $\m{f}_{i,e}$ of $\nabla f_i(\m{x}_{i, e}^k, \wh{\m{y}}^k)$
            	    \State $\m{x}_{i,e+1}^k = \m{x}_{i,e}^k - \alpha \m{f}_{i,e}$
        	    \EndFor
        	    \EndFor
    	    \EndFor
    	   % \State $\m{y}= \frac{1}{|\mathcal{S}|}\sum_{i \in \mathcal{S}} \Delta_i$
    	 \State $\m{y}^{t+1}= \m{y}^t-\frac{\beta}{|\mathcal{S}|}\sum_{i \in \mathcal{S}} (\m{y}^t -\m{y}_{i,E}^t)$
		\EndFor
\end{algorithmic}
\label{alg:fedopt}
\end{algorithm}
}
%%%
{
\small
\begin{algorithm}[htb]
\caption{\fedblo: A Federated Bi-Level Optimization Algorithm for Solving \eqref{fedblo:prob}.}
\label{alg:generalized_fedavg}
\begin{algorithmic}[1]
	    \State Input:  $(\m{x}_0, \m{y}_0)\in \mb{R}^{d_1}\times \mb{R}^{d_2}$; stepsizes $(\alpha,\beta)$
	    \For{$k = 0, \cdots, K-1$}
	        \State $\wh{\m{y}}^k~=~\pmb{\fedopt} (\m{x}^k, \m{y}^k)$
    	    \State Sample a subset $\mathcal{S}$ of clients
    	    \State $\m{x}_{i,0}^k = \m{x}^k$
    	    \For{each client $i \in \mathcal{S}$ \textbf{in parallel}}
        	    \For {$e = 0, \cdots, E-1$}
            	    \State Compute an unbiased estimate $\m{f}_{i,e}$ of $\nabla f_i(\m{x}_{i, e}^k, \wh{\m{y}}^k)$
            	    \State $\m{x}_{i,e+1}^k = \m{x}_{i,e}^k - \alpha \m{f}_{i,e}$
        	    \EndFor
    	    \EndFor
    	    \State $\m{x}^{k+1}=\m{x}^k-\frac{\alpha}{|\mathcal{S}|}\sum_{i \in \mathcal{S}} (\m{x}^k- \m{x}^k_{i, E})$
		\EndFor
\end{algorithmic}
\label{alg:fedopt}
\end{algorithm}
}
%
% \begin{algorithm}[t]
% \caption{\fedblo: A Federated Bi-Level Optimization Algorithm for Solving \eqref{fedblo:prob}.}
% %
% \begin{algorithmic}[1]\label{algo:fblo}
% \STATE Inputs: $x_0\in \mb{R}^{d_1}, y_0\in \mb{R}^{d_2}$; nonnegative sequences $\{\alpha_k\}_{k\ge 0}, \{\beta_t\}_{t\ge 0}$
% \FOR{$k=0, 1, \dots, K-1$}
% \FOR{$t=0, \dots, t_k-1$}
% \STATE Set $\tilde{y}_{i,0}= y_{0}.$
% \FOR{each client $i \in [n]$ \textbf{in parallel}}
% \FOR{$e = 0, \cdots, E-1$}
% \begin{equation}\label{eq:inner-problem-updates}
% y_{i,e+1}^{t}= y_{i,e}^{t}-\beta_t\nabla g_i(x_{i,k},y_{i,t}^{e-1}).
% \end{equation}   
% \ENDFOR
% \ENDFOR
% \STATE Set $ \tilde{y}_{i,k}=y_{i,t_k}$;
% \FOR{each client $i \in [n]$ \textbf{in parallel}}
% \FOR{$e = 0, \cdots, E-1$}
% \begin{equation} \label{eqn: outer_problem_update}
% % x_{i,k+1}=\sum_{j=1}^n[w]_{ij}^{\tau_2(k)} \left(x_{j,k}- \alpha_k \widetilde{\nabla} f_j(x_{j,k}, \tilde{y}_{j,k}(x_{j,k}))\right)
% x_{i,k+1}=\left(x_{j,k}- \alpha_k \widetilde{\nabla} f_j(x_{j,k}, \tilde{y}_{j,k})\right)
% \end{equation}
% \ENDFOR
% \ENDFOR
% \ENDFOR
% \ENDFOR
% \STATE Output: $x_{i,K},y_{i,K}$

% \end{algorithmic}
% \end{algorithm}

\section{Federated BiLevel Learning and \fedblo with Partial Information}\label{sec:fedavg:partial}

Next, we discuss how to define an appropriate approximation for the  gradient  of  the objective function $f$ in the outer problem. To do so, we recall how the \emph{implicit differentiation} formula of the gradient $\nabla \m{y}^*(\m{x})$ is obtained for smooth inner optimization problems \citep{bengio2000gradient}. The proof is provided in Appendix. 

% We will provide a generalization to non-smooth optimization problems in \Cref{sub:implicit_nonsmooth}.

To provide an iterative algorithm for solving problem \eqref{fedblo:prob}, we typically need to compute the gradient of $f$ at a given point $\m{x} \in  \mb{R}^{{d}_1}$ which requires knowing is not available unless the inner problem has a closed-form solution which is only possible for very specific choices of function $g$. Therefore, we assume that for any $\m{x} \in  \mb{R}^{{d}_1}$, we have an approximation of $\m{y}^*(\m{x})$ which is used to estimate the gradient of $f$ at $\m{x}$. More specifically, for any $\m{x} \in  \mb{R}^{{d}_1}$, we define the gradient approximation of $f$ as
\begin{eqnarray}\label{eq:approximate-gradient-nodewise}
\widetilde{\nabla} f_i\left(\m{x}_i,\tilde y_i\right) &:=& \nabla_{\m{x}}f_i\left(\m{x}_i,\tilde y_i\right)-
J_{i,w,\tau} (\m{x}_i,\tilde y_i) H^{-1}_{i,w,\tau} \left(\m{x}_i,\tilde y_i\right)
  \nabla_y f_i \left(\m{x}_i,\tilde y_i\right) 
  \nonumber \\
  &=& \nabla_{\m{x}}f_i\left(\m{x}_i,\tilde y_i\right)-
M_{i,w,\tau} (\m{x}_i,\tilde y_i) 
  \nabla_y f_i \left(\m{x}_i,\tilde y_i\right) 
\end{eqnarray}

%%%

\small
\begin{algorithm}[htb]
\caption{~\pmb{\fedblo}}
\label{alg:generalized_fedavg}
\begin{algorithmic}[1]
	    \State Input:  $(\m{x}^0, \m{y}^0)\in \mb{R}^{d_1}\times \mb{R}^{d_2}$; stepsizes $(\alpha, \{\beta\}_{i=1}^n)$;  $\m{H}^0 \in \mb{R}^{d_2\times d_2}$, $\m{J}^0 \in \mb{R}^{d_1\times d_2}$; compression operators $\mc{C}_c$ and $\mc{C}_s$; initial  $\m{H}_{i}^0=0, \m{J}_{i}^0=0~\forall i\in\mathcal{S}$.
\For{$k = 0, \cdots, K-1$}
%	         \State Generate  $\m{u}_{q}^k = N(0, \m{I}) \in \mb{R}^{d_1}$  for all $q =1, \ldots Q$ 
	        \State $ \m{y}^{k+1}~=~\pmb{\fedesj} (\m{x}^k, \m{y}^k, \beta, \mu)$
    	  %  \State Sample a subset $\mathcal{S}$ of clients
%    	    \State 
\For {$i \in \mc{S}$ \textbf{in parallel}} 
\For {$\ell=0,\ldots,\tau_i-1$} 
%\vspace{2mm}
\State $\m{x}^{k}_{i,\ell+1} \gets \m{x}^{k}_{i,\ell}-\alpha(\nabla_{\m{x}} f_i(\m{x}_{i,\ell}^k, \m{y}^{k+1})- \m{J}^k [\m{H}^k]^{-1}\nabla_\m{y} f_i(\m{x}_{i,\ell}, \m{y}^{t+1}))$; $\m{x}^k_{i,0}=\m{x}^k$
\EndFor
\EndFor
\For {$i \in \mc{S}$ \textbf{in parallel}} 
\State  $\m{S}_i^k=\mc{C}_c(\nabla^2_{\m{y}}g_i(\m{x}^k,\m{y}^k)- \m{H}_i^k)$ and  $\m{W}_i^k=\mc{C}_c(\nabla^2_{\m{xy}}g_i(\m{x}^k,\m{y}^k)- \m{H}_i^k)$ 
\State  $\m{H}_i^{k+1} = \m{H}_i^k + \pi_1 \m{S}_i^k$ and $\m{J}_i^{k+1} = \m{J}_i^k + \pi_2\m{W}_i^k$;
%\State Send $\nabla f_i(x^k)$,\; $\mS_i^k \eqdef \cC_i^k(\nabla^2 f_i(x^k) - \mH_i^k)$ and $l_i^k \eqdef \|\mH_i^k - \nabla^2 f_i(x^k)\|_{\rm F}$ to the server
\EndFor
\State  $\m{S}^k=\mc{C}_s( 1/m\sum_{i=1}^m \m{S}_i^k)$ and  $\m{W}^k=\mc{C}_s(1/m\sum_{i=1}^m \m{W}_i^k)$ 
\State  $\m{H}^{k+1} = \m{H}^k + \pi_1 \m{S}^k$ and $\m{J}^{k+1} = \m{J}^k + \pi_2\m{W}^k$;
%\State Send $\nabla f_i(x^k)$,\; $\mS_i^k \eqdef \cC_i^k(\nabla^2 f_i(x^k) - \mH_i^k)$ and $l_i^k \eqdef \|\mH_i^k - \nabla^2 f_i(x^k)\|_{\rm F}$ to the server
\EndFor
\end{algorithmic}
\label{alg:fedopt}
\end{algorithm}

{
\small
\begin{algorithm}[htb]
\caption{~\pmb{\fedblo}: A Federated Bi-Level Optimization Algorithm for Solving \eqref{fedblo:prob}.}
\label{alg:generalized_fedavg}
\begin{algorithmic}[1]
	    \State Input:  $(\m{x}^0, \m{y}^0)\in \mb{R}^{d_1}\times \mb{R}^{d_2}$; stepsizes $(\alpha,\beta)$
	    \For{$k = 0, \cdots, K-1$}
	         \State Generate  $\m{u}_{q}^k = N(0, \m{I}) \in \mb{R}^{d_1}$  for all $q =1, \ldots Q$ 
	  %  \For{q=0, \ldots, Q}   
	        \State $ (\m{y}^{k+1},\{\wh{\delta}^k_{q}\}_{q=1}^Q)~=~\pmb{\fedesj}
	        (\m{x}^k, \m{y}^k, \{\m{u}_{q}^k\}_{q=1}^Q,\beta, \mu)$
            %	  \EndFor
    	    \State Sample a subset $\mathcal{S}$ of clients
    	    \State $\m{x}_{i,0}^k = \m{x}^k$
    	    \For{each client $i \in \mathcal{S}$ \textbf{in parallel}}
        	    \For {$e = 0, \cdots, E-1$}
            	    \State Compute  $\wh{\nabla} \phi (\m{x}_{i,e}^k) = \nabla_x f_i(\m{x}_{i,e}^k, \m{y}^{k+1}, \zeta^k_i)+\frac{1}{Q}\sum_{q=1}^Q \langle \nabla_x f_i(\m{x}^k,\m{y}^{k+1};\xi^k_i), \wh{\g{\delta}}^k_q\rangle \m{u}_{q}^k$
            	    \State $\m{x}_{i,e+1}^k = \m{x}_{i,e}^k - \alpha \wh{\nabla} \phi (\m{x}_{i,e}^k)$
        	    \EndFor
    	    \EndFor
    	    \State $\m{x}^{k+1}= \frac{1}{|\mc{S}|}\sum_{i \in \mathcal{S}} \m{x}^k_{i, E}$
		\EndFor
\end{algorithmic}
\label{alg:fedopt}
\end{algorithm}
}

{
\small
\begin{algorithm}[htb]
\caption{$ (\m{y}^T,\{\delta^T_{q}\}_{q=1}^Q) ~=~\pmb{\fedesj} (\m{x},\m{y}^0, \{\m{u}_q\}_{q=1}^Q, \beta,`\mu)$}
\label{alg:generalized_fedavg}
\begin{algorithmic}[1]
	    %\State Input: 
	    \State  $\m{y}_{q}^0=\m{y}^{0}$ for all $q =0, \ldots Q$ and $\m{u}_{0} = \m{0}$
	    \For{$t=0,\cdots,T-1$}
	        	    \State Sample a subset $\mathcal{S}$ of clients
    	    \State  $\m{y}_{i,0,q}^t=\m{y}_{q}^{t}$
    	    \For{each client $i \in \mathcal{S}$ \textbf{in parallel}}
        	    \For {$e = 0, \cdots, E-1$}
	    	    \For{q=0, \ldots, Q}            	    \State $\m{y}_{i,e+1,q}^t=\m{y}_{i,e,q}^t-\beta \nabla g_i(\m{x}+ \mu \m{u}_{q}, \m{y}_{i,e,q}, \zeta_{i}^t)$
        	    \EndFor
        	    \EndFor
             \State $\m{y}_{q}^{t+1}=  \frac{1}{|\mathcal{S}|}\sum_{i \in \mathcal{S}} \m{y}_{i,E,q}^t$ 
    	    \EndFor
    	    \State   $\delta^T_{q}= \frac{\m{y}^{T}_{q}-\m{y}_{0}^T}{\mu}$  for all $q =1, \ldots Q$. 
    	    \EndFor 
    	 \end{algorithmic}
\label{alg:fedopt}
\end{algorithm}
}

{\small
\begin{algorithm}[t]
\caption{~\fedblo
%\colorbox{red!30}{\pmb{$\fedblo$}}, \colorbox{green!30}{\pmb{$\fedminmax$}}, and \colorbox{blue!20}{\pmb{$\fedcomp$}} 
}
\label{alg:fedblo}
\begin{algorithmic}[1]
	    \State Input:  $(\m{x}^0, \m{y}^0)\in \mb{R}^{d_1}\times \mb{R}^{d_2}$; stepsizes $(\alpha, \{\beta_i\}_{i=1}^n)$.
	    %$\m{H}^0 \in \mb{R}^{d_2\times d_2}$; compression operators $\mc{C}_s$ and $\mc{C}_c$ ; initial  $\m{H}_{i}^0=0 ~\forall i\in\mathcal{S}$.
\For{$k = 0, \cdots, K-1$}
\For {$t=0,\ldots,T-1$} 
\State $\m{y}^{k,t+1} ~=~\pmb{\fedsvrg}(\m{x}^k,\m{y}^{k,t}, q^{k,t}, \{\beta_i\}_{i=1}^m)$
 \For {$i \in \mc{S}$ \textbf{in parallel}} 
\State Compute $\nabla_y g_i(\m{x}, \m{y}^{k,t+1})$
\EndFor
\State $q^{k,t+1}=1/m\sum_{i\in\mathcal{S}}\nabla_y g_i(\m{x}, \m{y}^{k,t+1})$
%\State $ \m{y}^{k+1} ~=~\pmb{\fedsvrg}(\m{x}^k, \m{y}^{k}, \{\beta_i\}_{i=1}^m)$
% \For {$i \in \mc{S}$ \textbf{in parallel}} 
% %\State  Compute $$
% %$\m{S}_i^k=\mc{C}_c(\nabla^2_{\m{y}}g_i(\m{x}^k,\m{y}^{k+1})-\m{H}_i^k)$, and $\m{H}_i^{k+1} = \m{H}_i^k + \pi \m{S}_i^k$
% %\State Send $\nabla f_i(x^k)$,\; $\mS_i^k \eqdef \cC_i^k(\nabla^2 f_i(x^k) - \mH_i^k)$ and $l_i^k \eqdef \|\mH_i^k - \nabla^2 f_i(x^k)\|_{\rm F}$ to the server
% \EndFor 
%\State  %$\nabla_\m{y} f(\m{x}^k, \m{y}^{k+1})=$;
%\State {Set $r_Q = 1/m\sum_{i\in\mathcal{S}} \nabla_{\m{y}} g_i(\m{x}^k, \m{y}^{k+1})$}
\EndFor
		\For{$t=T-1,...,0$}
		\For {$i \in \mc{S}$ \textbf{in parallel}} 
		 \State \textbf{If} $t=T-1$, $\m{p}_{i}^{k,t}=\nabla_{\m{y}}^2 g_i(\m{x}^k, \m{y}^{k,t+1}) $ \textbf{else} $\m{p}_{i}^{k,t}=\m{p}^{k,t+1}-\beta_i \nabla_\m{y}^2  g_i (\m{x},\m{y})\m{p}^{k,t+1}$ 
		\EndFor
		\State $\m{p}^{k,t}= 1/m\sum_{i\in\mathcal{S}} \m{p}_{i}^t$
	%\State { $\m{p}^{k}=\sum_{t=0}^{T-1}\m{p}^{k,t}$}
		%		\STATE{Set $z_j=r_0$}
%		\ENDFOR
		\EndFor
		\State { $\m{p}^k=\sum_{t=0}^{T-1}\m{p}^{k,t}$}
%$\m{H}^{k+1} =\mc{C}_s\left(\m{H}^k+ \pi/m\sum_{i\in\mathcal{S}}\m{S}_i^k\right)$
%\State $\m{p}^k~=~\pmb{\fedgrad}(\nabla_y f(\m{x}^k, \m{y}^{k+1})$
%\State $\m{p}^k~=~\pmb{\fedgrad}(\nabla_y f(\m{x}^k, \m{y}^{k+1}))$
%\For {$i \in \mc{S}$ \textbf{in parallel}} 
%\State $\m{x}^k_{i,0}=\m{x}^k$
%\For {$\ell=0,\ldots,\tau_i-1$} 
%\vspace{2mm}
%\State $\m{x}^{k}_{i,\ell+1} \gets \m{x}^{k}_{i,\ell}-\alpha_i\left( \nabla_{\m{x}} f_i(\m{x}_{i,\ell}^k, \m{y}^{k+1})- \nabla_{\m{x}} f_i(\m{x}^k, \m{y}^{k+1})  + \m{p}^k \right)$; $\m{x}^k_{i,0}=\m{x}^k$
%\m{J}^k [\m{H}^k]^{-1}\nabla_\m{y} f_i(\m{x}_{i,\ell}, \m{y}^{t+1}))$; 
%\EndFor
%\EndFor
%\State $\m{x}^{k+1}=1/m\sum_{i\in\mathcal{S}}\m{x}^k_{i,\tau_i}$
%\State 
 \For {$i \in \mc{S}$ \textbf{in parallel}} 
 \State $ \m{x}_{i}^k= \m{x}^k_i- \alpha (\nabla_{\m{x}} f_i(\m{x}^k, \m{y}^{k,T}) - \sum_{t=0}^{T-1}\nabla^2_{\m{xy}}g_i(\m{x}^k,\m{y}^{k,t}) \m{p}^k) $
% \State  $\m{H}_i^{k+1} = \m{H}_i^k + \pi_1 \m{S}_i^k$ and $\m{J}_i^{k+1} = \m{J}_i^k + \pi_2\m{W}_i^k$;
% %\State Send $\nabla f_i(x^k)$,\; $\mS_i^k \eqdef \cC_i^k(\nabla^2 f_i(x^k) - \mH_i^k)$ and $l_i^k \eqdef \|\mH_i^k - \nabla^2 f_i(x^k)\|_{\rm F}$ to the server
\EndFor
\State  $\m{x}^{k+1}=1/m\sum_{i\in\mathcal{S}}\m{x}_{i}^k$
 \EndFor
\end{algorithmic}
\label{alg:fedopt}
\end{algorithm}
}
