# Supplementary material for: FedNest: Federated Bilevel, Minimax, and Compositional Optimization
Source: arXiv:2205.02215 source file (2022-09-13)
Supplement: Supplementary file 4 [file supp_ntable.tex]

\begin{table}
	\centering
	{\caption{Summary of the Notations}~\label{tab:notation}
	{\footnotesize \begin{tabular}{l l l }
		\toprule
		\bfseries Constant & \bfseries Description & \bfseries Reference \\
		\midrule 
% 		$L_{fx}, L_{fy}$ & Lipschitz constants for $\nabla_x f(x,\cdot)$, $\nabla_y f(x,\cdot)$ w.r.t.~$y$, resp. & %\Cref{ass:f}
% 		\\
% 		$\bar{L}_{fy}$ & Lipschitz constants for $\nabla_y f(\cdot,y)$ w.r.t.~$x$ & %\Cref{ass:f} 
% 		\\
% 		$C_{fy}$ & Upper bound on $\| \nabla_y f(x,y) \|$ & %\Cref{ass:f}
% 		\\
% 		$L_g$ & Lipschitz constant of $\nabla_y g(x,\cdot)$ & 
% 		%\Cref{ass:g} 
% 		\\
% 		$\mu_g$ & Strong convexity modulus $g(\m{x},\cdot)$ w.r.t.~$\m{y}$ & %\Cref{ass:g}
% 		\\
% 		$L_{gxy}, L_{gyy}$ & Lipschitz constants of $\nabla_{xy}^2g(x,\cdot), \nabla_{yy}^2 g(x,\cdot)$ w.r.t.~$y$, resp. & %\Cref{ass:g} 
% 		\\
% 		$\bar{L}_{gxy}, \bar{L}_{gyy}$ & Lipschitz constants of $\nabla_{xy}^2 g(\cdot,y), \nabla_{yy}^2 g(\cdot,y)$ w.r.t.~$x$, resp. & %\Cref{ass:g} 
% 		\\
% 		$C_{gxy}$ & Upper bound on $\| \nabla_{xy}^2 g(x,y) \|$ & %\Cref{ass:g}
%		\\
%		$\sigma_g^2, \sigma_f^2$ & Variance of stochastic estimates $\m{q}(\m{x},\m{y})$, $\m{h}(\m{x},\m{y})$, resp. & Assumptions~\ref{assu:bound:var}, \ref{assu:bound:var:minmax}, 
%		\ref{assu:bound:var:compos}
%		\\
		$\tilde\sigma_f^2$ & Constant term on the bound for $\bar{\m{h}}_i (\m{x}_{i,\nu}, \m{y})=\mb{E}\left[\m{h}_i(\m{x}_{i,\nu}, \m{y}^+)|{\cal F}_{i,\nu-1}\right]$ & Lemmas~\ref{lem:lips}, \ref{lem:lips:minmax},  \ref{lem:lips:compos} %\eqref{eq:hfbd} 
		\\
		$b$ & Bound on the bias of $\bar{\m{h}}(\m{x},\m{y})$ & Lemma~\ref{lem:neum:bias} %\Cref{ass:stoc} 
		\\
		$M_f$ & Difference between each $\bar{\nabla} f_i(\m{x},\m{y})$ and  $\nabla f_i (\m{x},\m{y}^*(\m{x}))$ w.r.t.~$\| \m{y}^\star(\m{x})-\m{x}\|$ &Lemmas~\ref{lem:lips}, \ref{lem:lips:minmax},  \ref{lem:lips:compos}
		\\
		$L_y$ & Lipschitz constant of $\m{y}^\star(\m{x})$ &Lemmas~\ref{lem:lips}, \ref{lem:lips:minmax},  \ref{lem:lips:compos}
		\\
		$L_f$ & Lipschitz constant of $\nabla f(\m{x})$ &Lemmas~\ref{lem:lips}, \ref{lem:lips:minmax},  \ref{lem:lips:compos}
		\\
		$L_{yx}$ & Lipschitz constant of $\nabla \m{y}^\star(\m{x})$ &Lemmas~\ref{lem:lips}, \ref{lem:lips:minmax},  \ref{lem:lips:compos}
		\\
		\bottomrule
	\end{tabular} }}
\end{table}
