# Supplementary material for: FedNest: Federated Bilevel, Minimax, and Compositional Optimization
Source: arXiv:2205.02215 source file (2022-09-13)
Supplement: Supplementary file 14 [file supp_localfedout.tex]

\begin{algorithm}[t]
\caption{$\m{x}^{+} ~=~\pmb{\fedout}~(\m{x}, \m{y}, \alpha)$ for stochastic \colorbox{cyan!30}{bilevel}, \colorbox{green!30}{min-max}, and \colorbox{magenta!30}{compositional} problems
} %\colorbox{purple!30}{SVRG}}
\begin{algorithmic}[1]
\State $\funco_i(\cdot)\gets \nabla_\m{x} f_i(\cdot,\m{y};\cdot)$
%\colorbox{cyan!30}{$\nabla_\m{y} f_i(\cdot)$~\text{(bilevel)}}, \colorbox{green!30}{$-\nabla_\m{y} f_i(\cdot)$~\text{(min-max)}},\\ \hspace{35pt}\colorbox{magenta!30}{$-h_i(\cdot)$~\text{(composite)}}%\func_i\gets 
 \State $\m{x}_{i,0}=\m{x}$ and $\alpha_i \in (0,\alpha]$
\State \colorbox{cyan!30}{Choose $N\geq 1$ and set $ \m{p}_N=~\pmb{\fedhess}~(\m{x}, \m{y},N)$}
 \For{$i \in \mc{S}$ \textbf{in parallel}} 
 \State \colorbox{cyan!30}{$\m{h}_i= \funco_i(\m{x};\xi_{i})-\nabla^2_{\m{xy}}g_i(\m{x},\m{y};{\zeta}_{i})
 \m{p}_N$}
 \State \colorbox{green!30}{$\m{h}_i=\funco_i(\m{x};  \xi_{i})$}
% \State \colorbox{magenta!30}{$\m{h}_i= \nabla h_i(\m{x};  \zeta_{i}) \nabla f_i(\m{y};  \xi_{i})$}
 \EndFor
 \State $\m{h}=|\mathcal{S}|^{-1}\sum_{i\in\mathcal{S}}\m{h}_i$

 \For {$i \in \mc{S}$ \textbf{in parallel}} 
\For {$\ell=0,\ldots,\tau_i-1$} 
 %\State Choose $\beta_i \in (0, \beta)$
% \For {$i \in \mc{S}$ \textbf{in parallel}} 
 \State%\colorbox{cyan!30}{
$\m{h}_{i,\ell}=\funco_i(\m{x}_{i,\ell}; \xi_{i,\ell})-\funco_i(\m{x}; \xi_{i,\ell})+\m{h}$
 %}%\colorbox{purple!30}{SVRG}
% \State \colorbox{red!30}{$ \m{h}_{i,\ell}= \nabla_{\m{x}} f_i(\m{x}, \m{y}^*(\m{x}))-\nabla^2_{\m{xy}}g_i(\m{x},\m{y}^*(\m{x}))
% \m{p}_N $}-%\colorbox{purple!30}{SVRG}
% \State\colorbox{green!30}{$\m{h}_{i,\ell}=\nabla_{\m{x}} f_i(\m{x}_{i,\ell}, \m{y}; \xi_{i,\ell})-\nabla_{\m{x}} f_i(\m{x}, \m{y}; \xi_{i,\ell})$}%\colorbox{purple!30}{SVRG}
%\State \colorbox{magenta!30}{$\m{h}_{i,\ell}=-\nabla_y f_i(\m{x}, \m{y};  \xi_{i})$}
 %\State \colorbox{magenta!30}{$\m{h}_i=\nabla h_i(\m{x}_{i,\ell};  \zeta_{i,\ell}) \nabla f_i(\m{y}_{i,\ell};  \xi_{i,\ell})-\nabla h_i(\m{x}; \zeta_{i,\ell}) \nabla f_i(\m{y};  \xi_{i,\ell})$}
 %~~\Comment{via automatic differentiation}
% \State  $\m{H}_i^{k+1} = \m{H}_i^k + \pi_1 \m{S}_i^k$ and $\m{J}_i^{k+1} = \m{J}_i^k + \pi_2\m{W}_i^k$;
% %\Stae Send $\nabla f_i(x^k)$,\; $\mS_i^k \eqdef \cC_i^k(\nabla^2 f_i(x^k) - \mH_i^k)$ and $l_i^k \eqdef \|\mH_i^k - \nabla^2 f_i(x^k)\|_{\rm F}$ to the server
%\State  $\m{x}^{+}=1/m\sum_{i\in\mathcal{S}}\m{x}_{i}$
 \State  $ \m{x}_{i,\ell+1}= \m{x}_{i,\ell}- \alpha_i\m{h}_{i,\ell}$%~~\Comment{via automatic
  \EndFor
\EndFor
\State $\m{x}^{+}=|\mc{S}|^{-1}\sum_{i\in \mc{S}} \m{x}_{i,\tau_i}$
% \EndFor
\end{algorithmic}
\label{alg:localfedout}
\end{algorithm}
